# Supplementary material for: Sequential Dexterity: Chaining Dexterous Policies for Long-Horizon Manipulation
Source: arXiv:2309.00987 source file (2023-10-16)

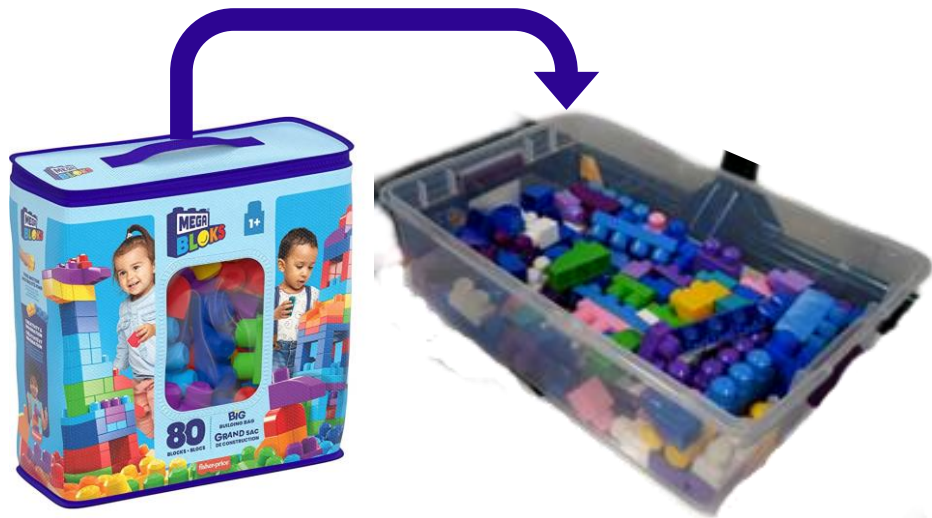

(a) Real world

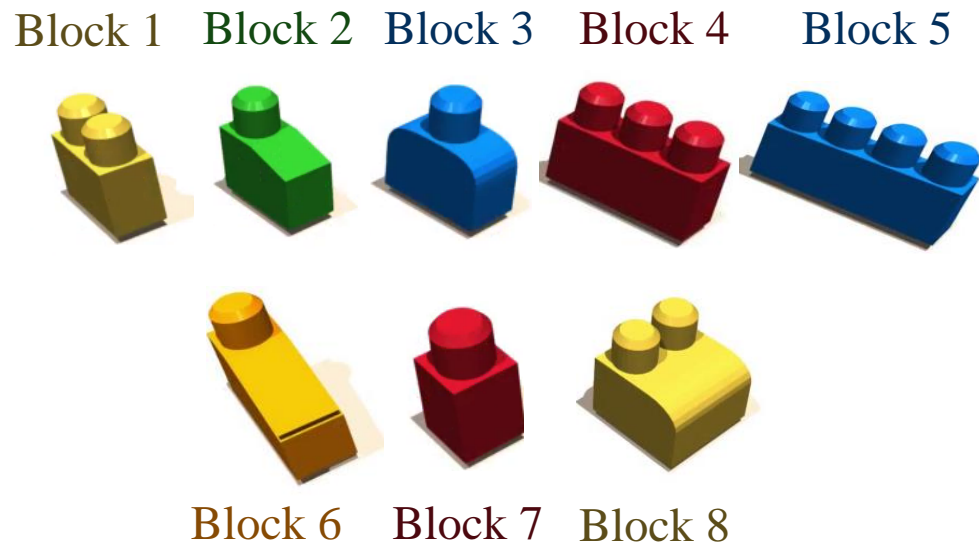

(b) Simulation

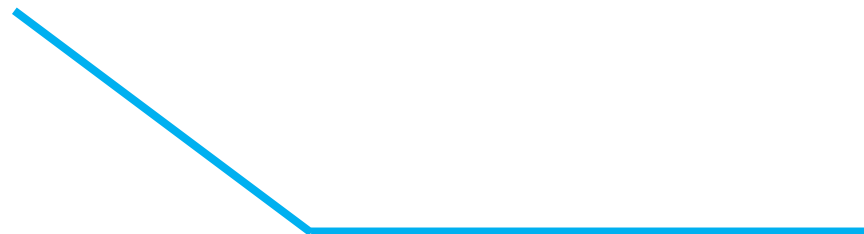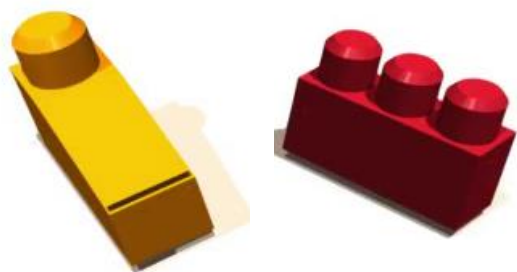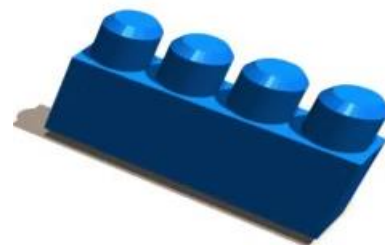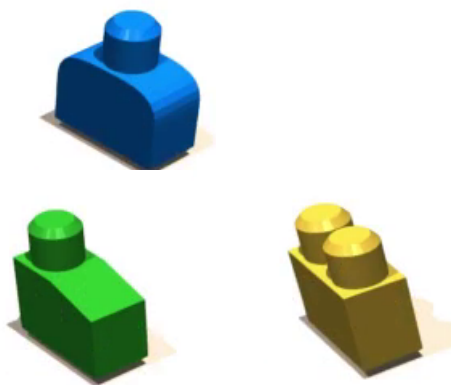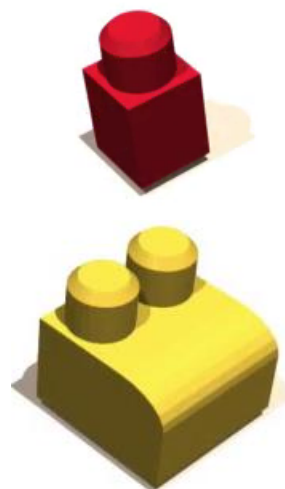

Supplement: Supplementary file 1 [file mega_bloks.pdf]
